# Supplementary material for: VQFR: Blind Face Restoration with Vector-Quantized Dictionary and Parallel Decoder
Source: arXiv:2205.06803 source file (2022-07-27)
Supplement: Supplementary file 1 [file lfw1.pdf]

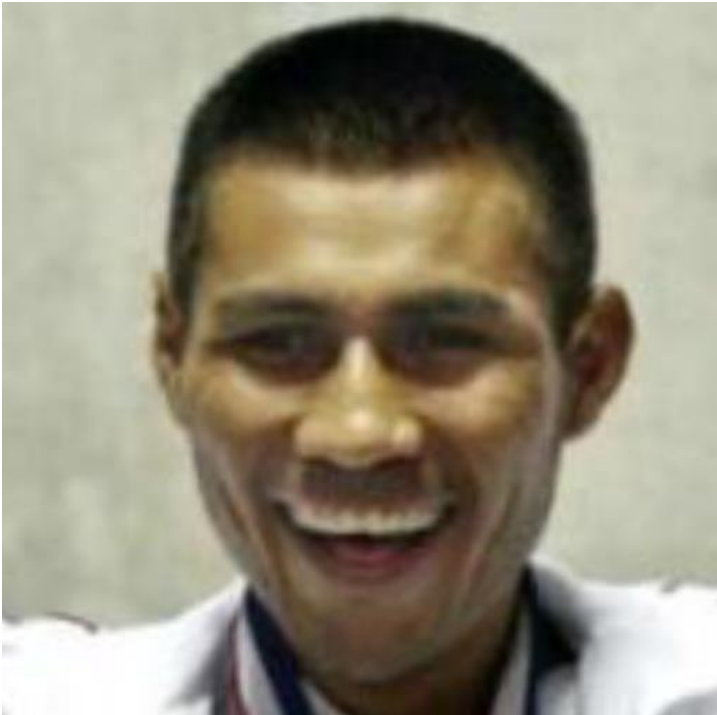

Input

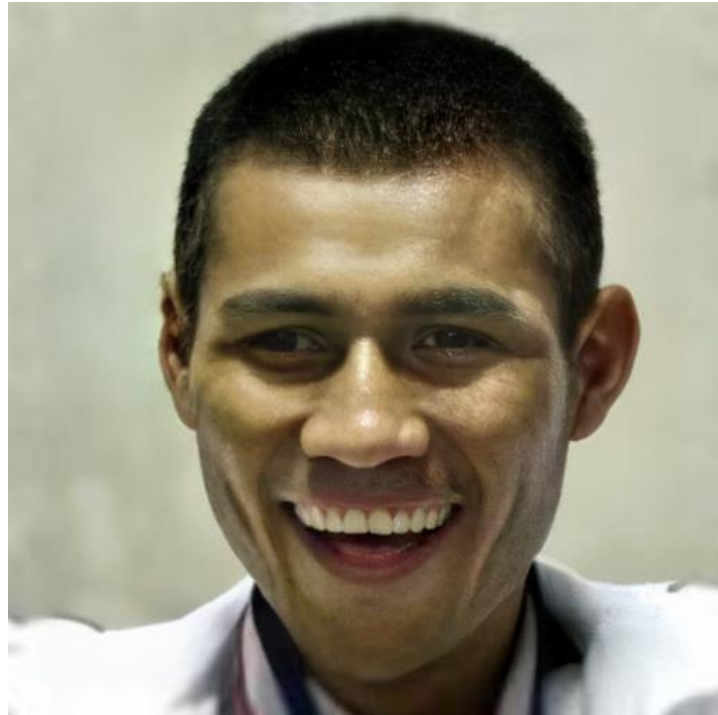

DFDNet

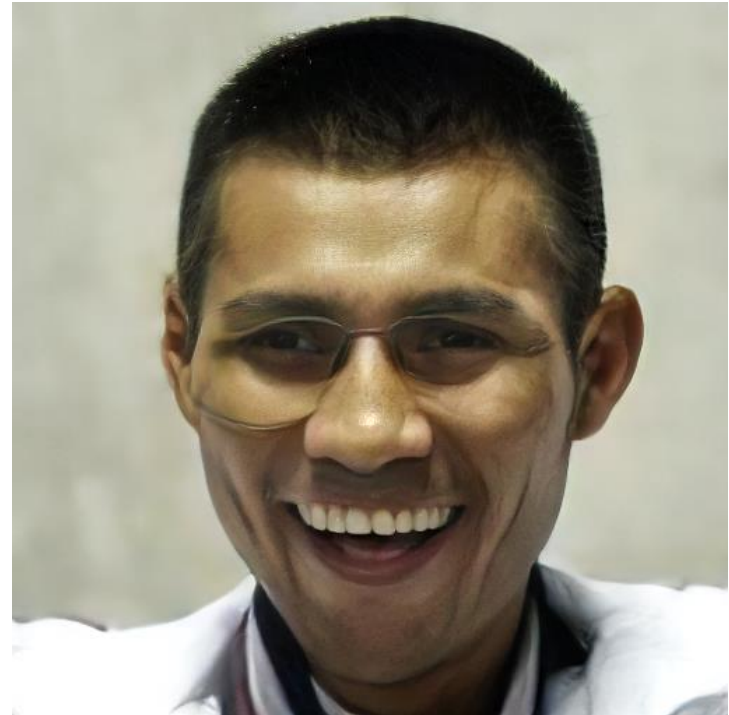

PSFRGAN

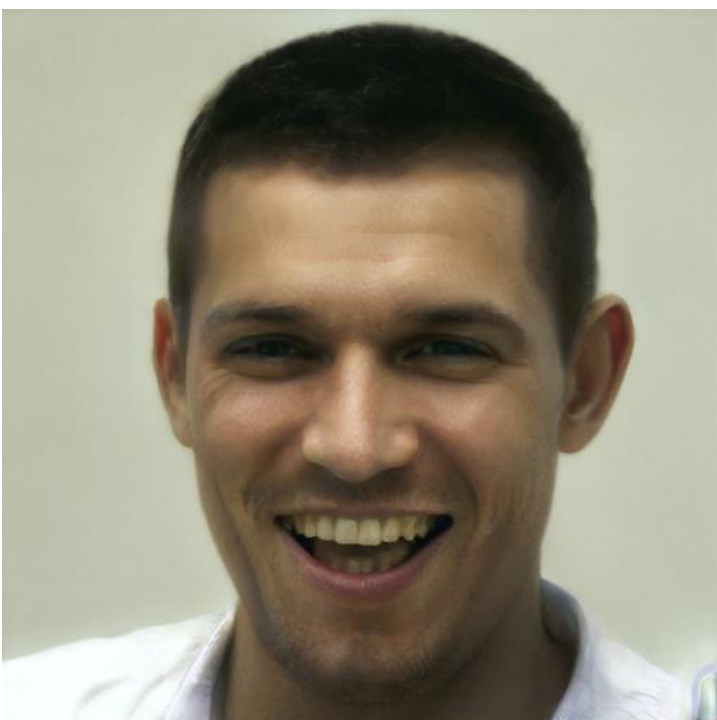

PULSE

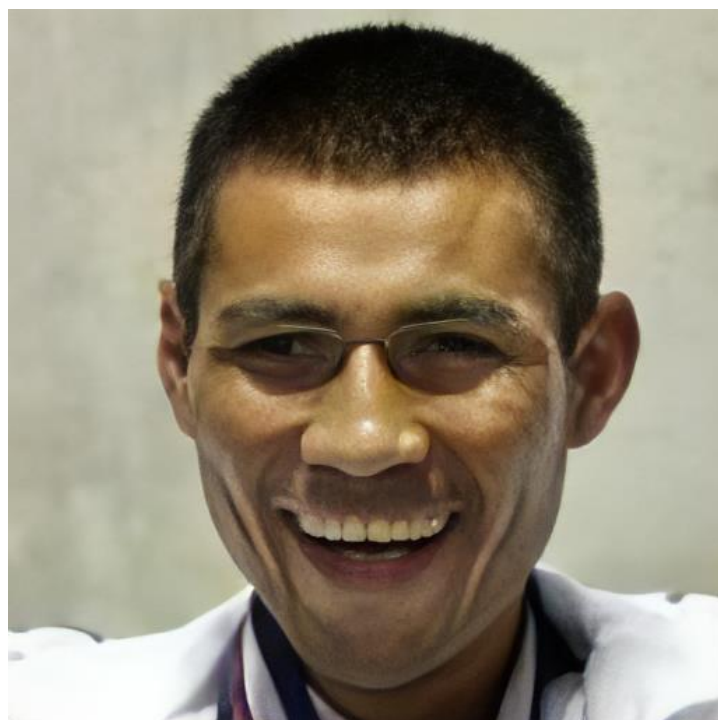

GFP-GAN

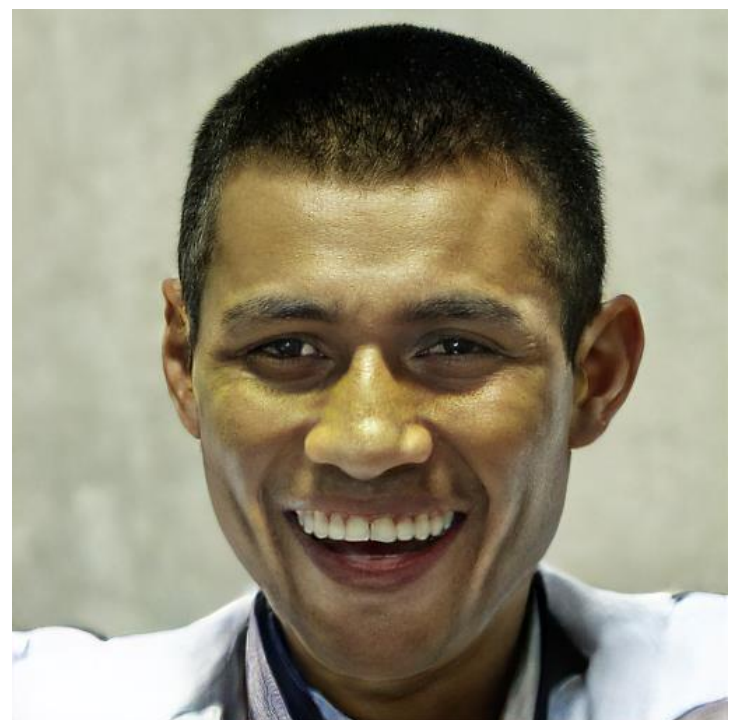

VQFR(ours)

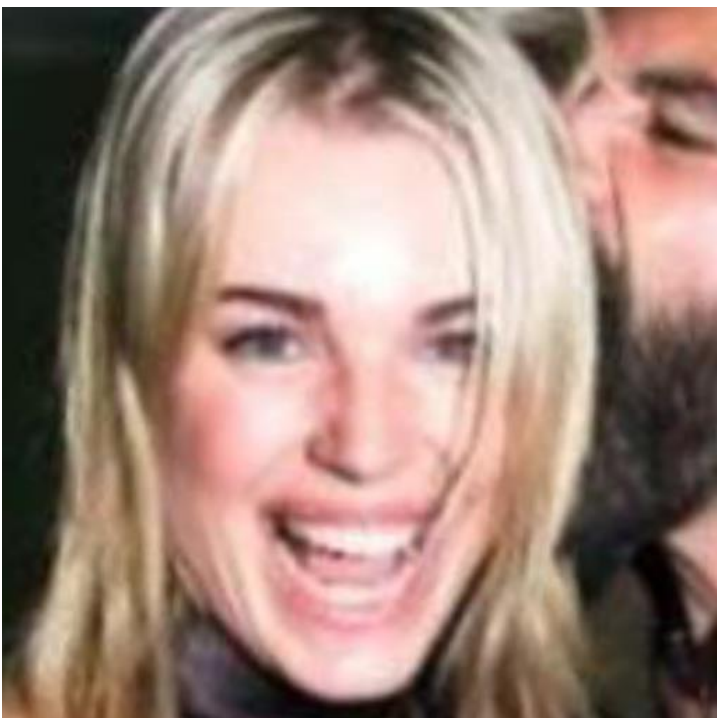

Input

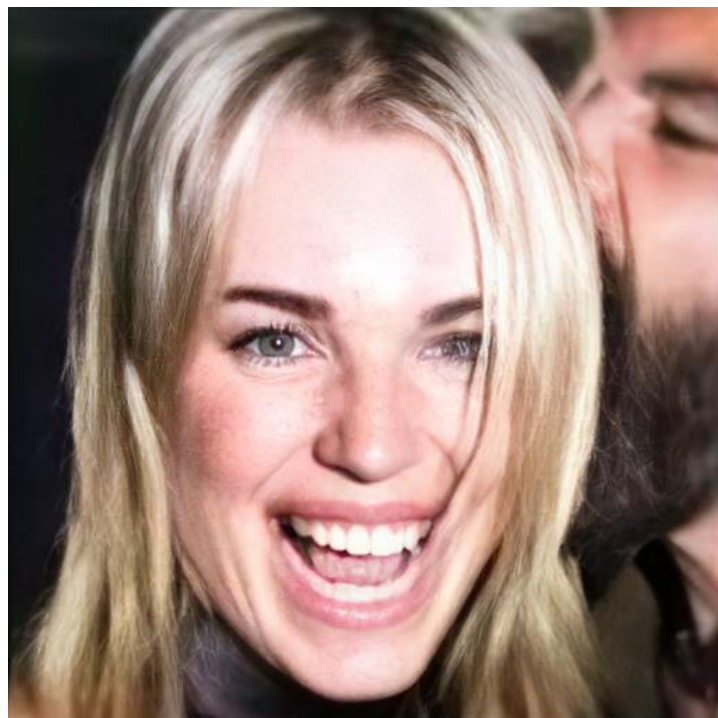

DFDNet

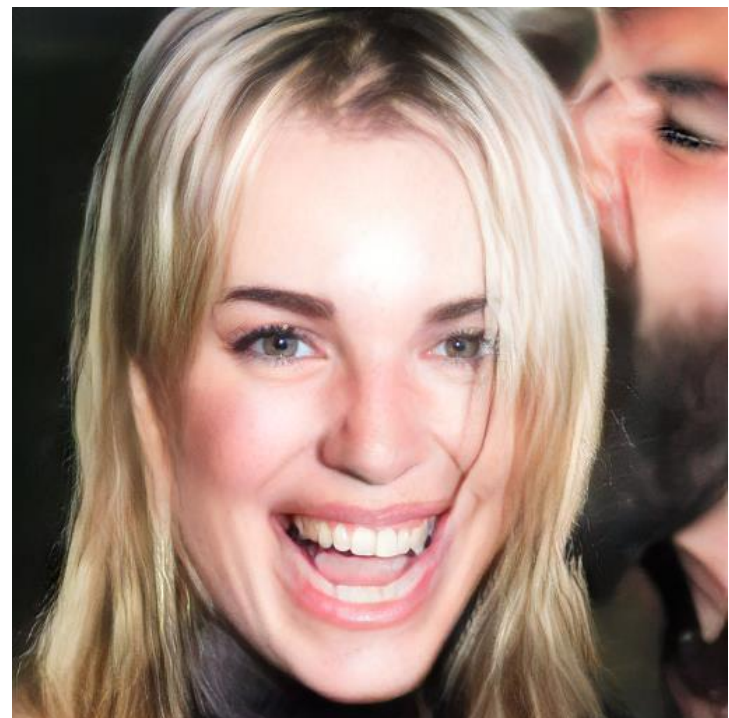

PSFRGAN

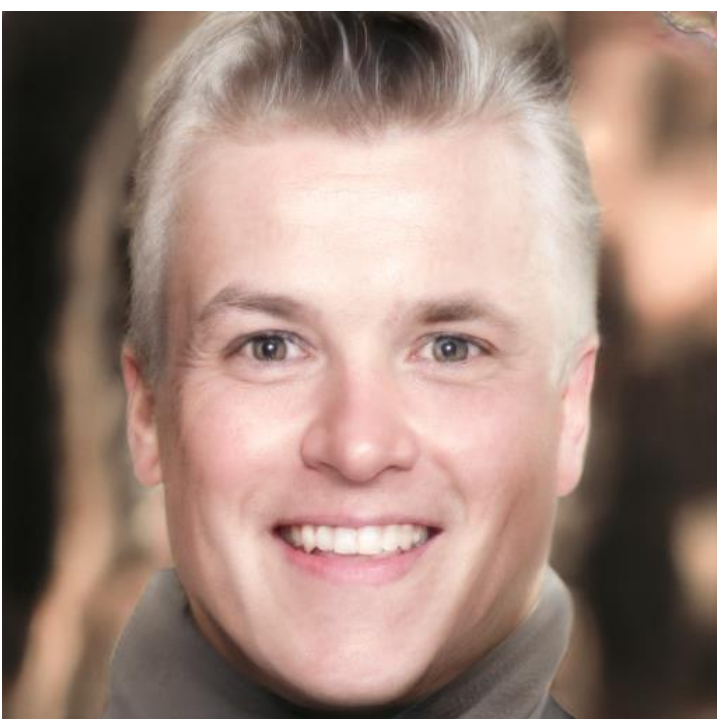

PULSE

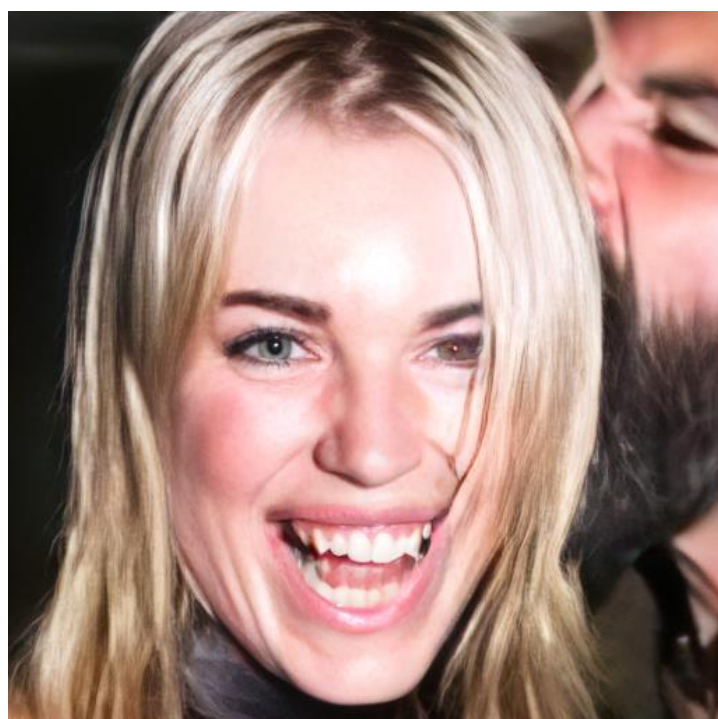

GFP-GAN

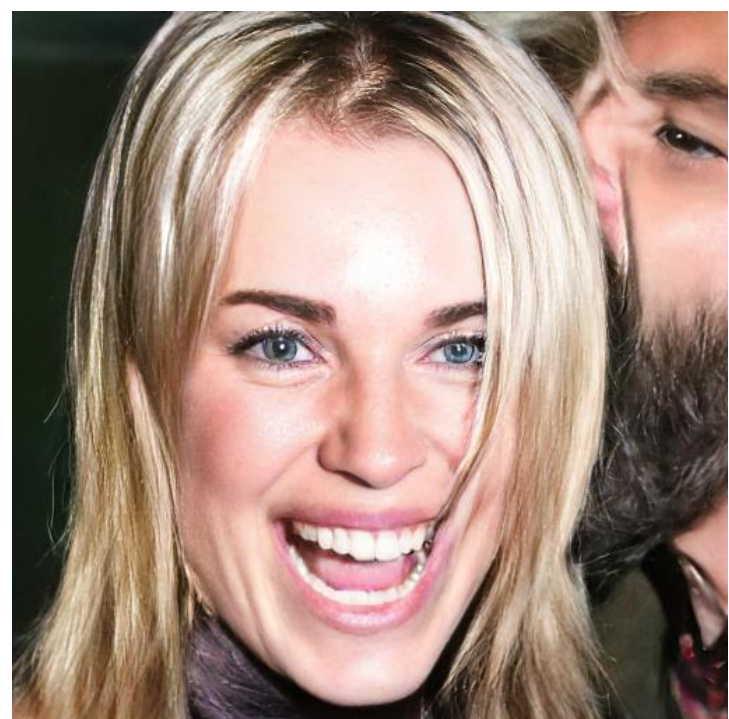

VQFR(ours)



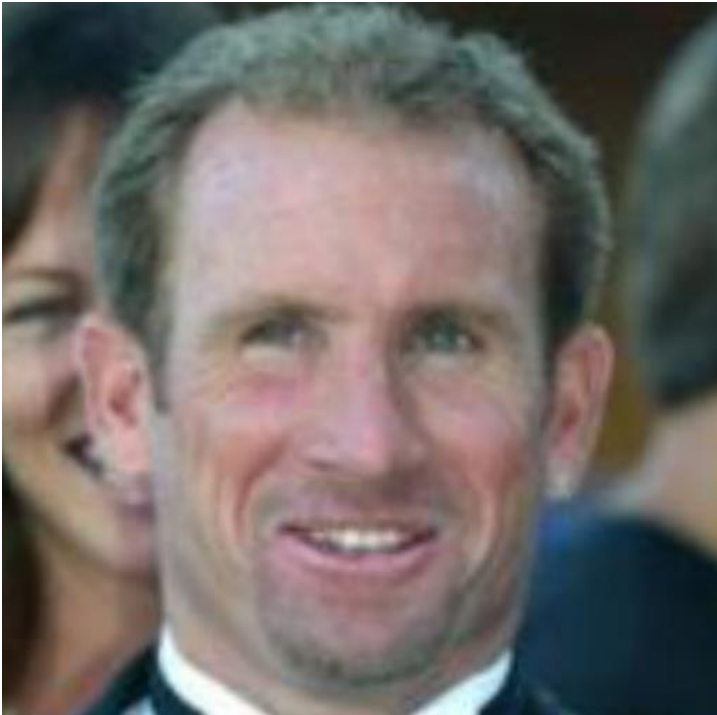

Input

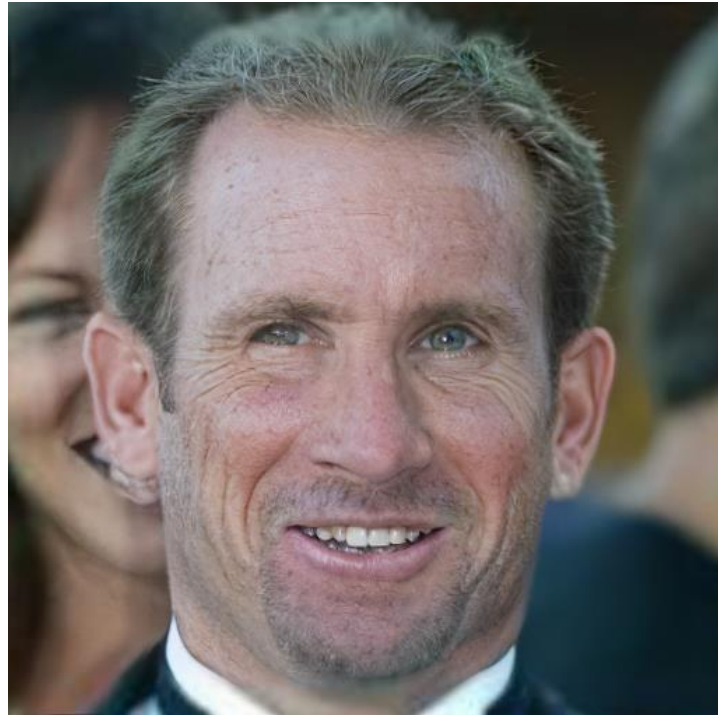

DFDNet

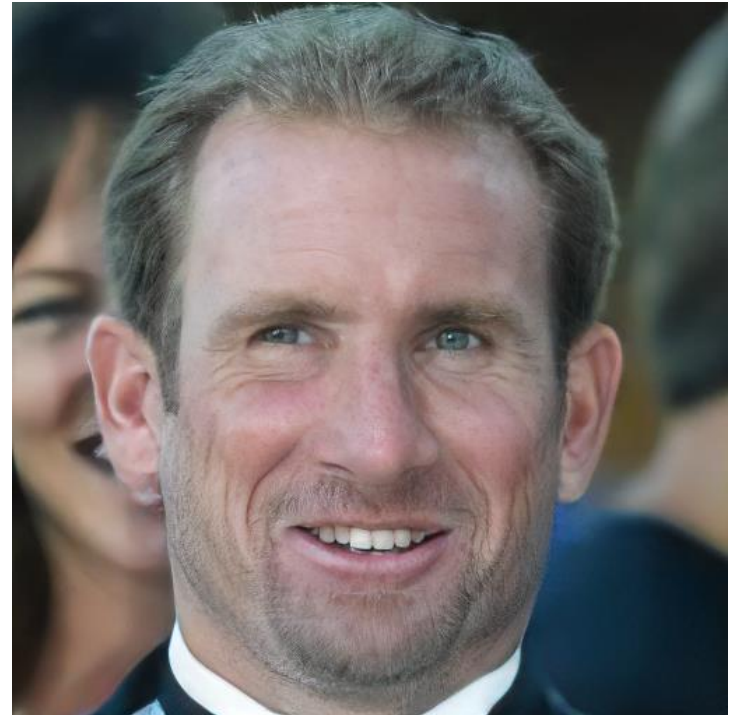

PSFRGAN

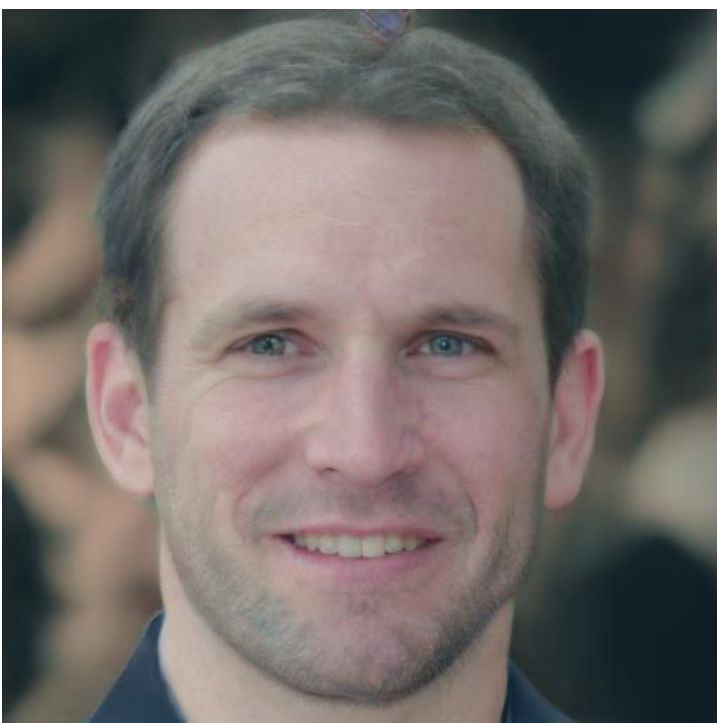

PULSE

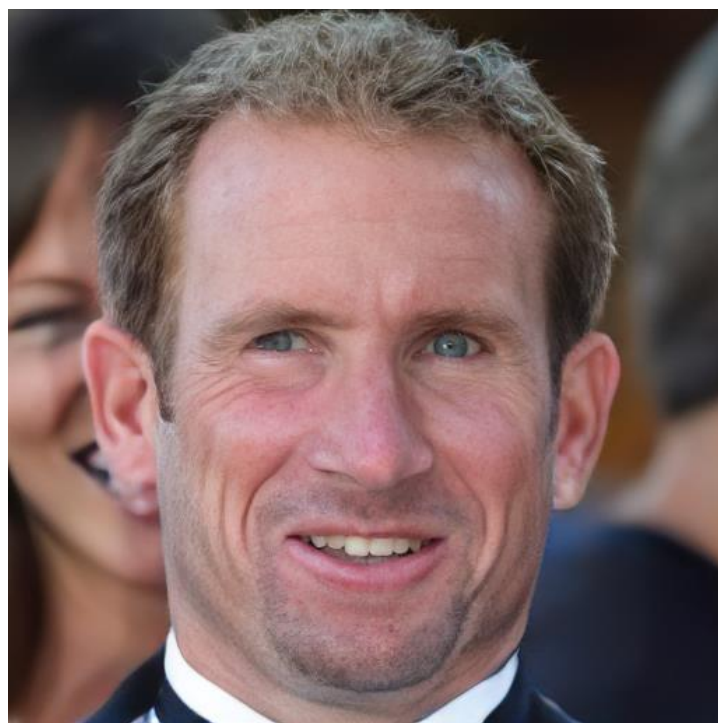

GFP-GAN

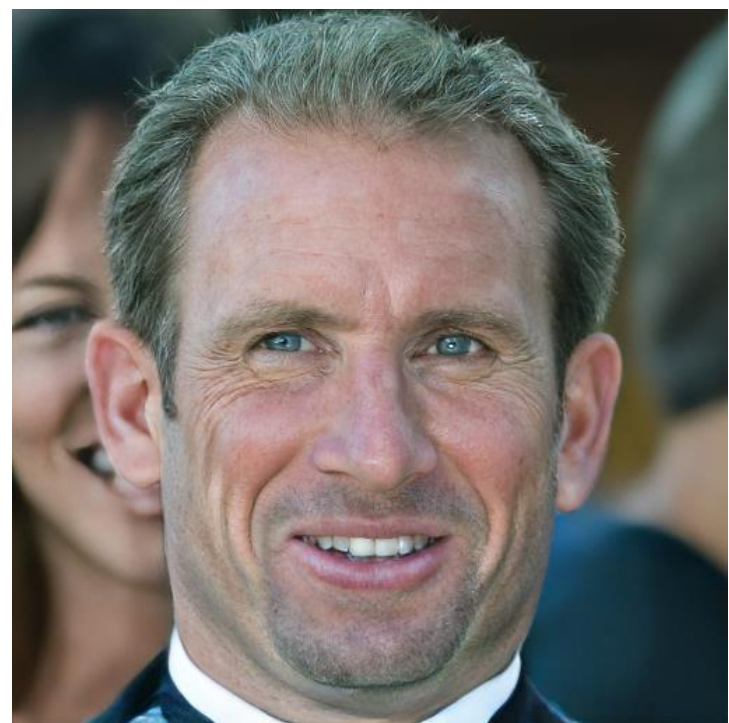

VQFR(ours)

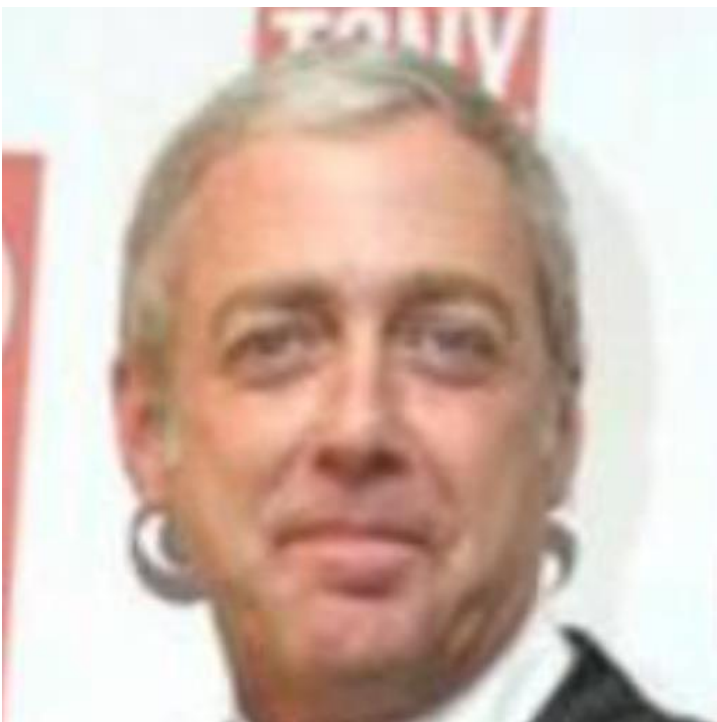

Input

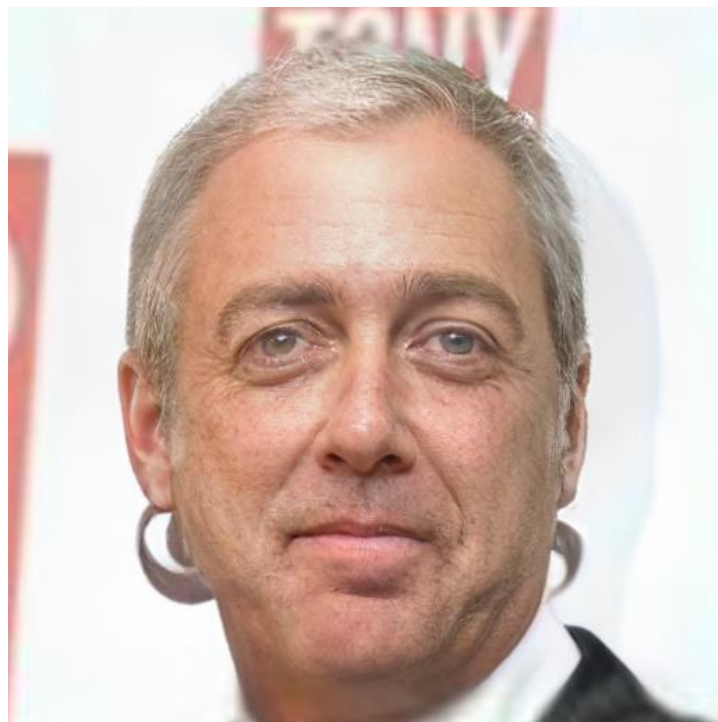

DFDNet

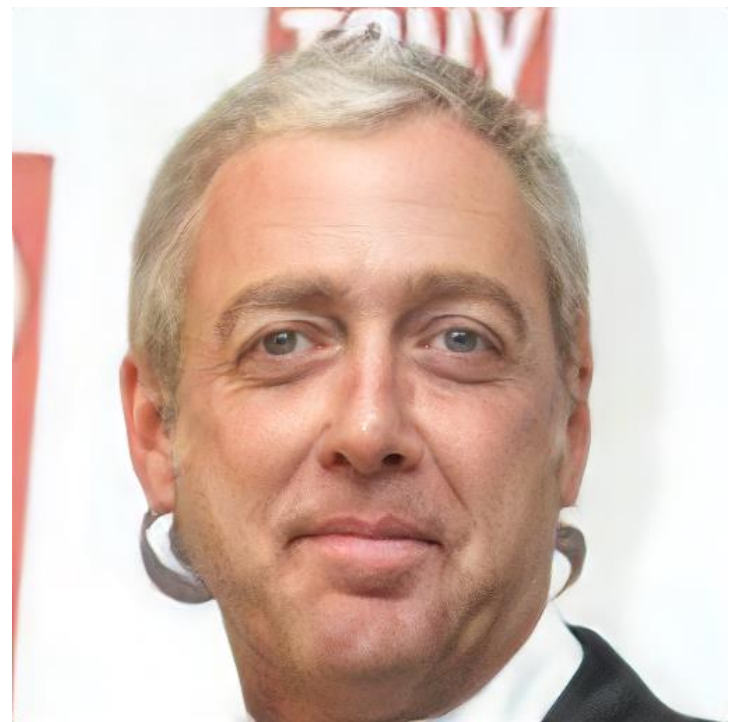

PSFRGAN

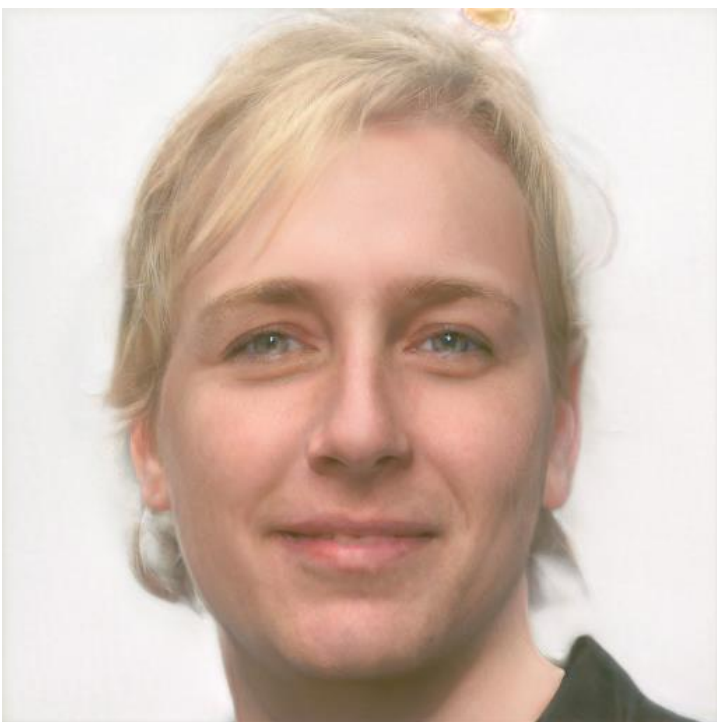

PULSE

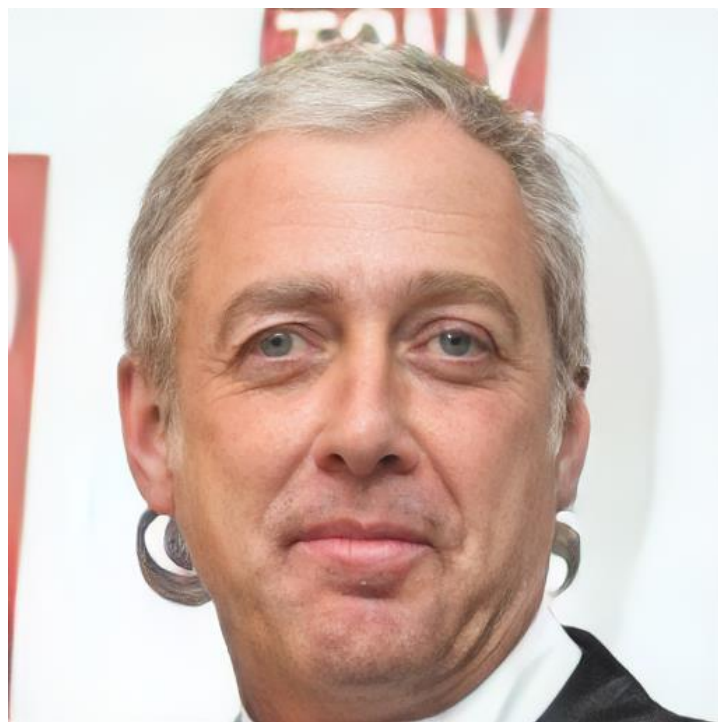

GFP-GAN

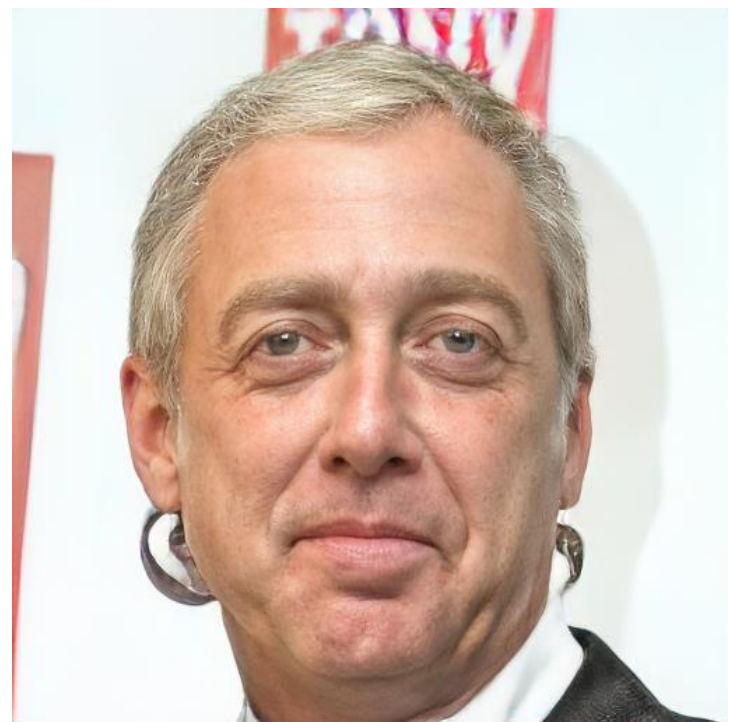

VQFR(ours)



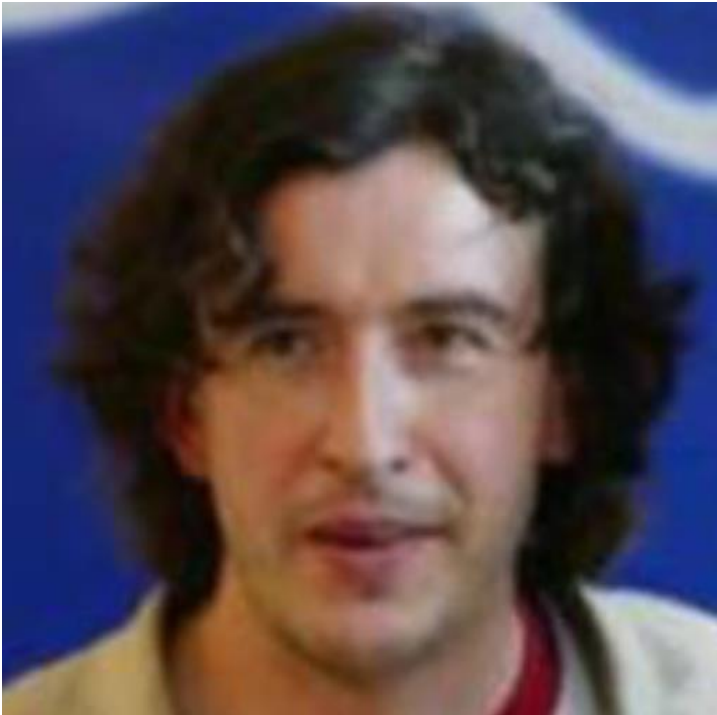

Input

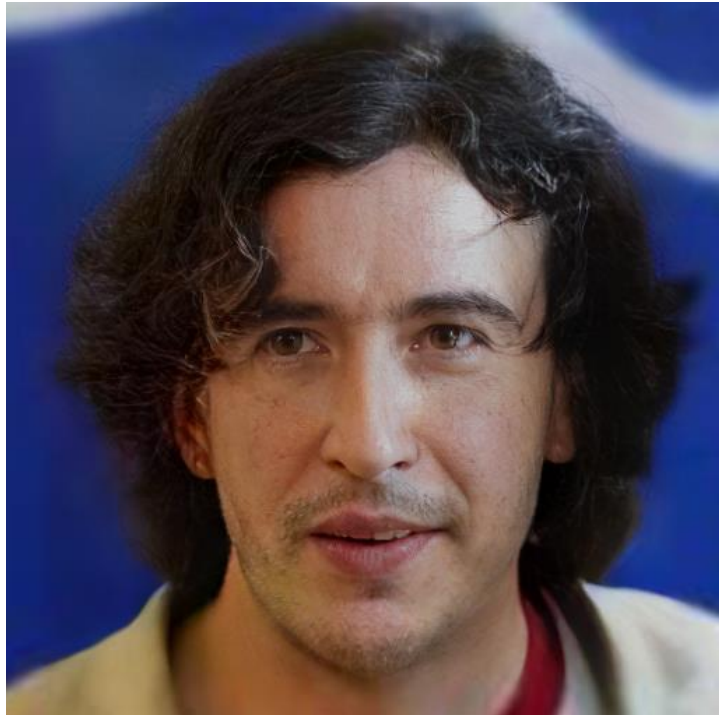

DFDNet

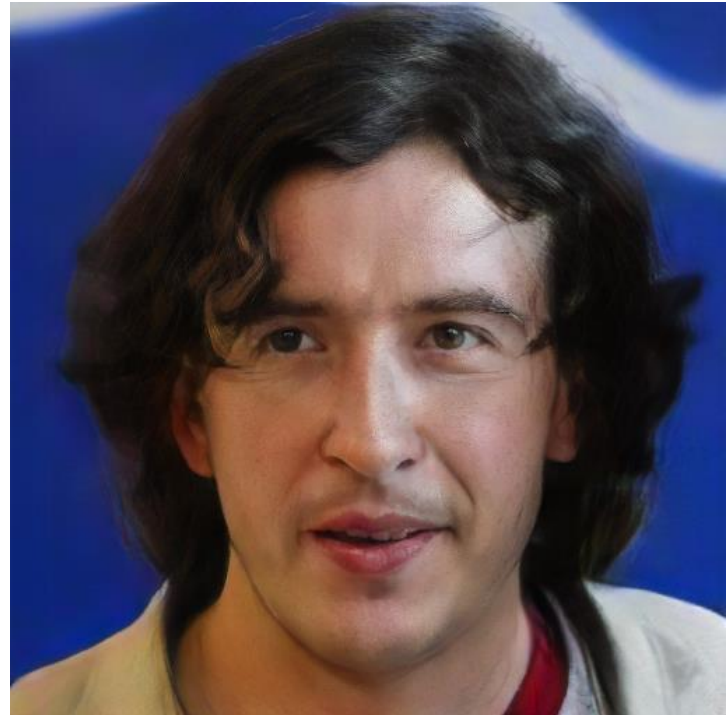

PSFRGAN

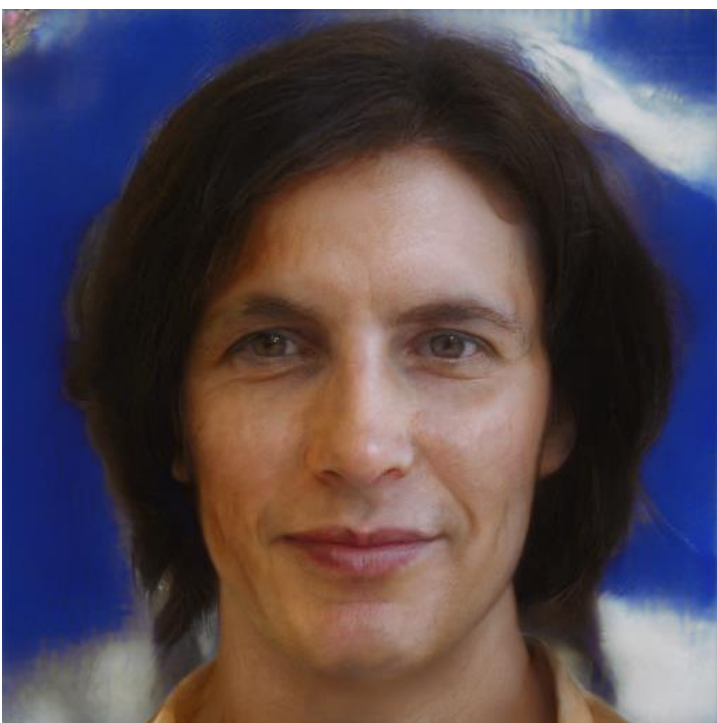

PULSE

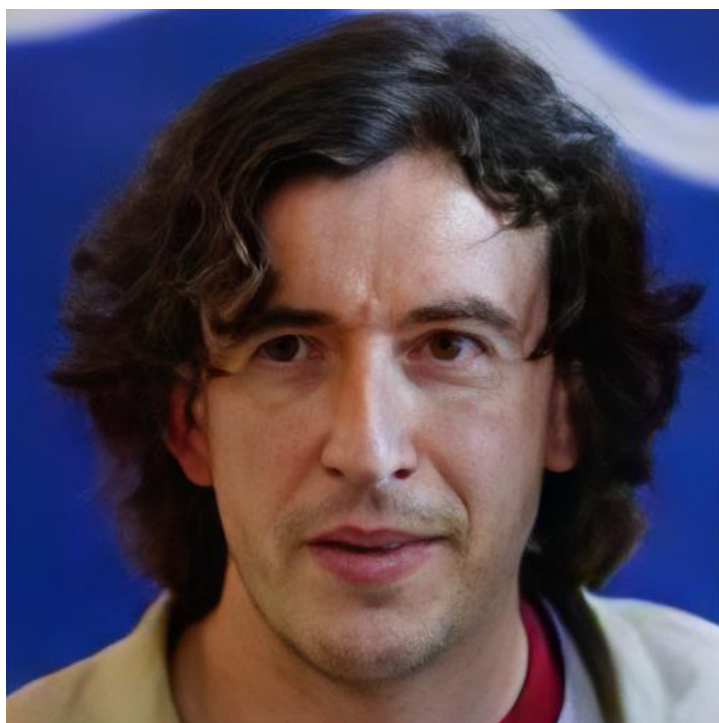

GFP-GAN

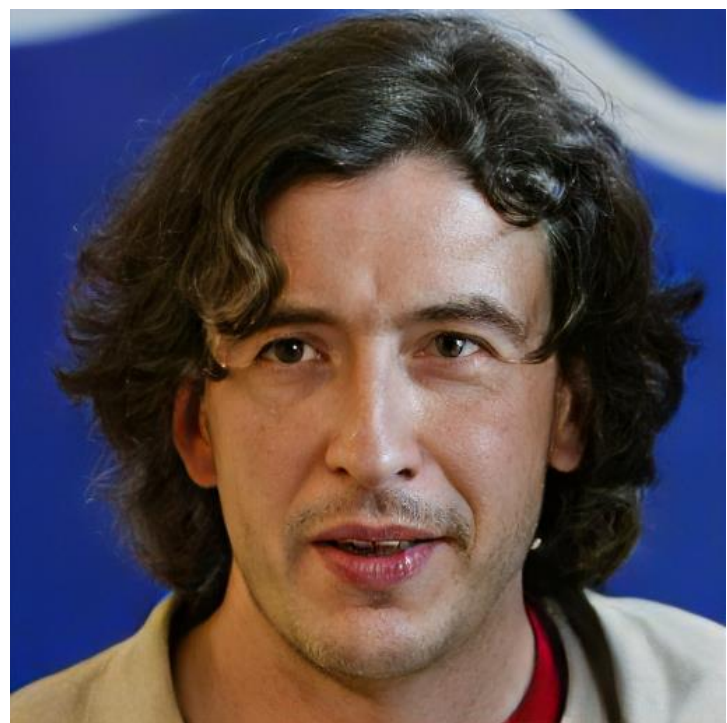

VQFR(ours)

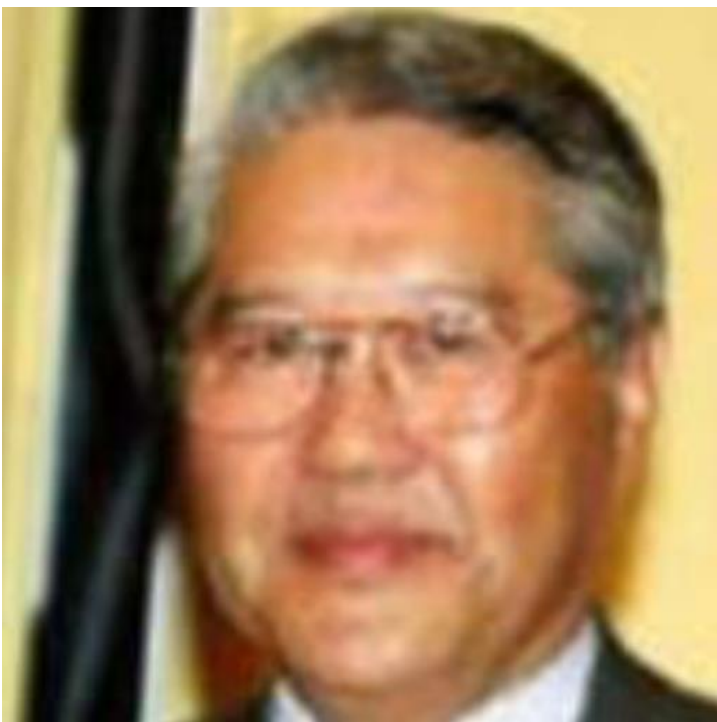

Input

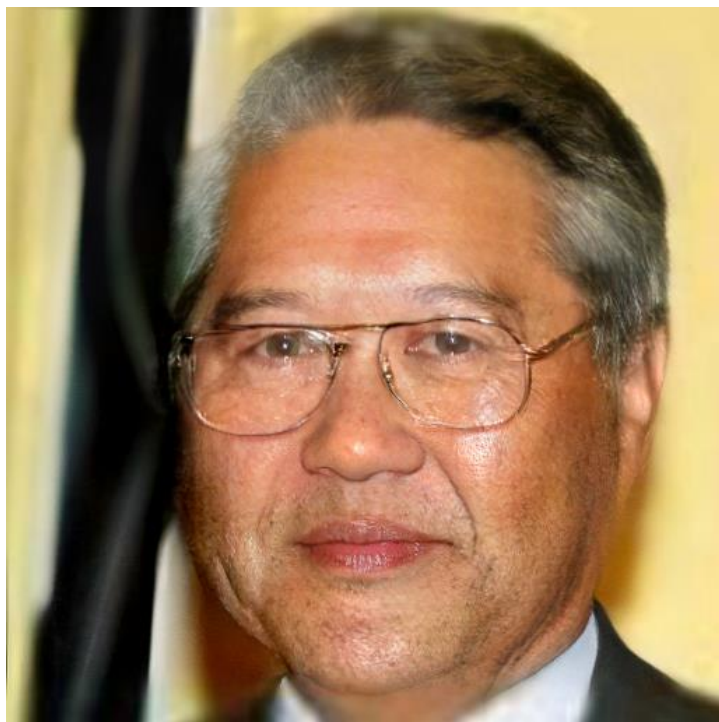

DFDNet

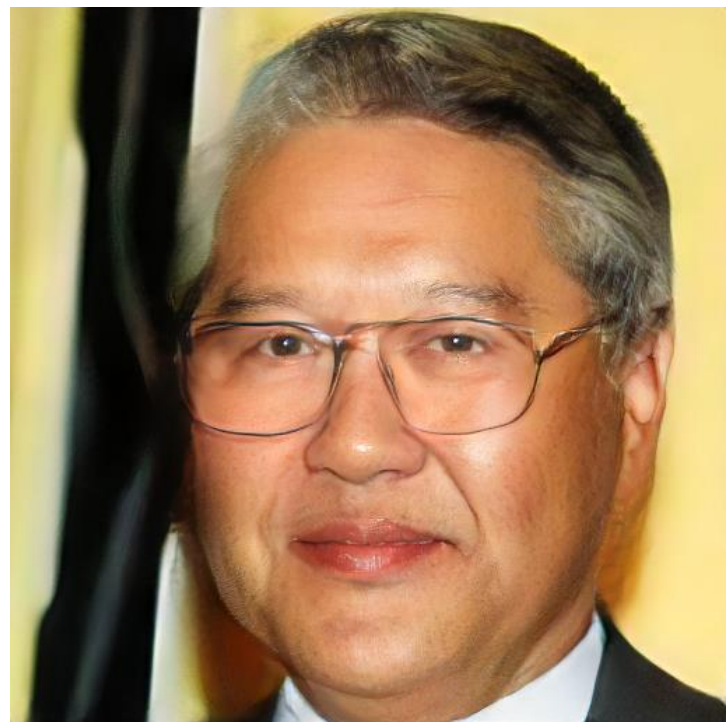

PSFRGAN

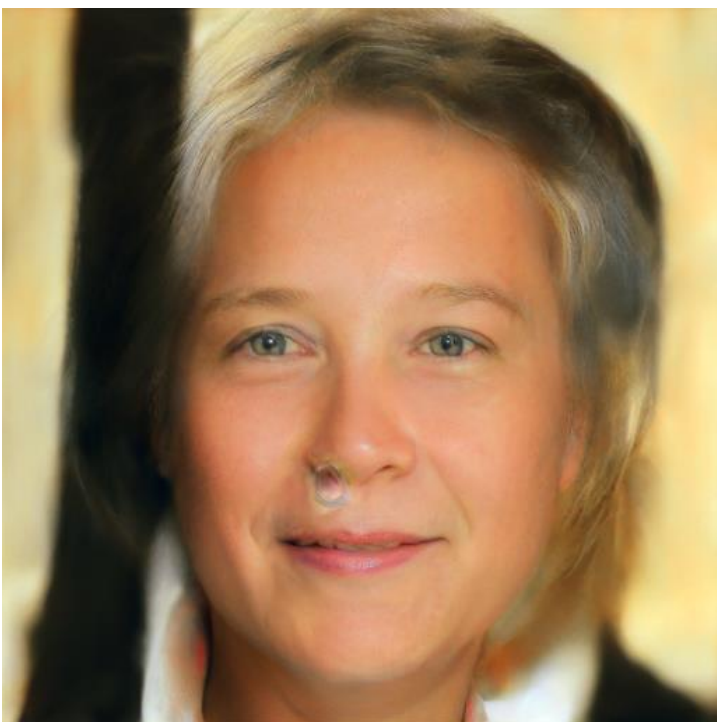

PULSE

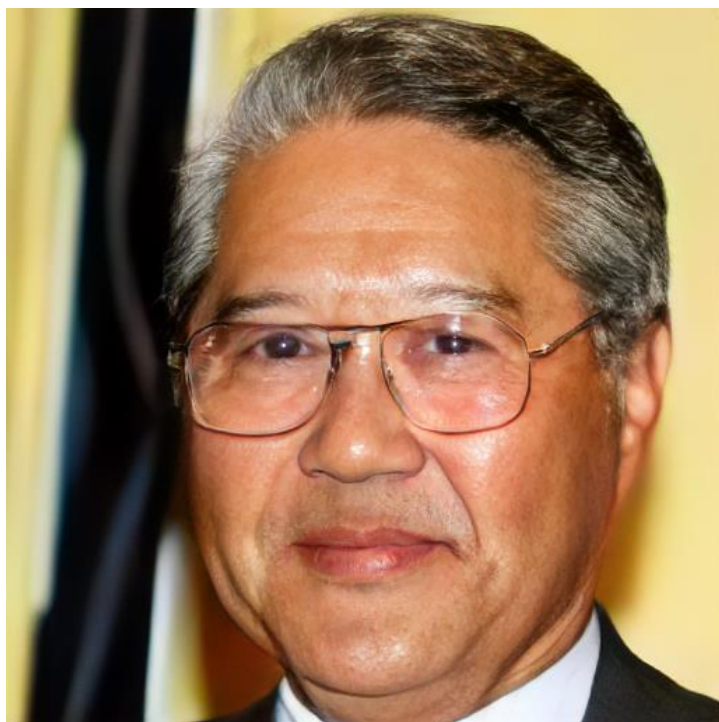

GFP-GAN

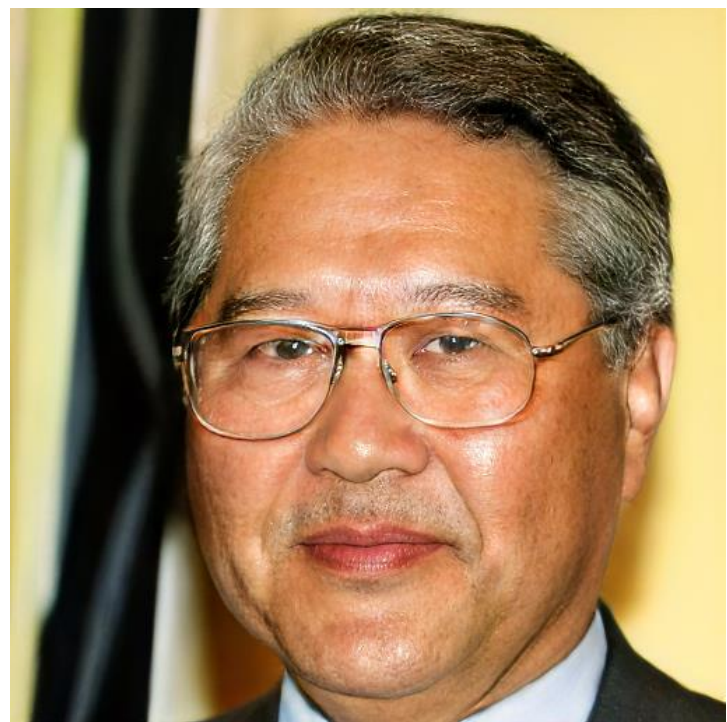

VQFR(ours)



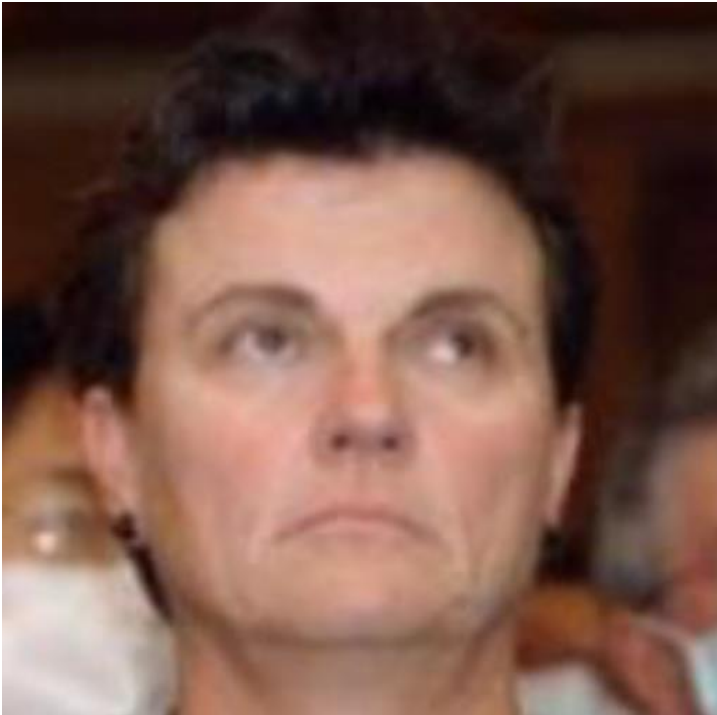

Input

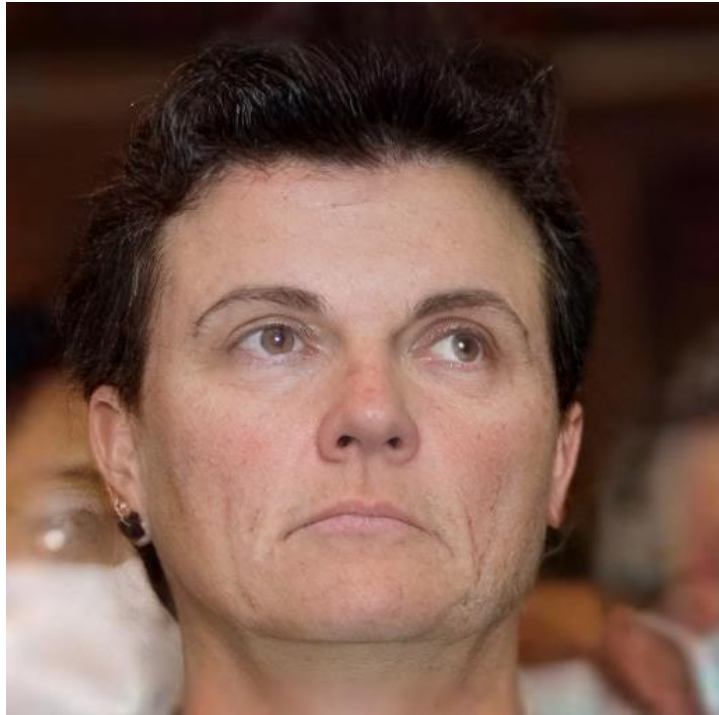

DFDNet

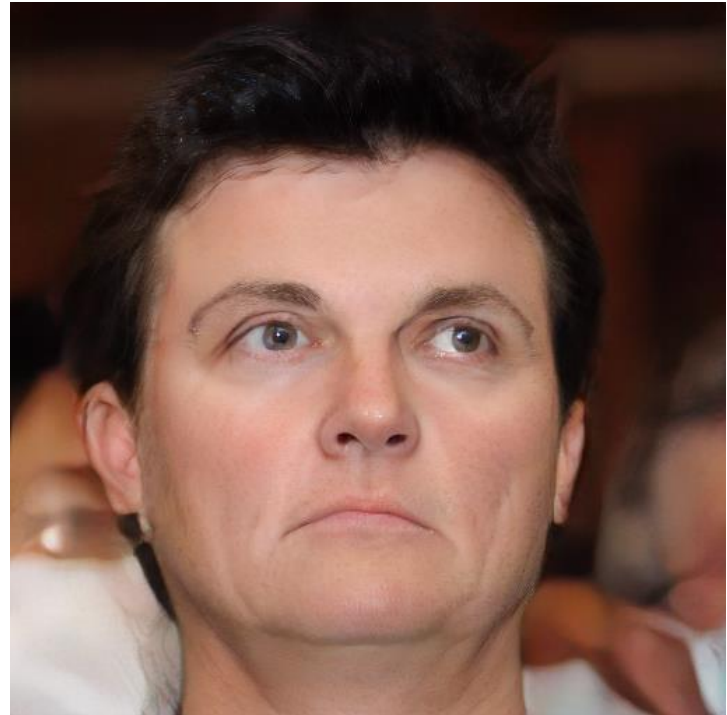

PSFRGAN

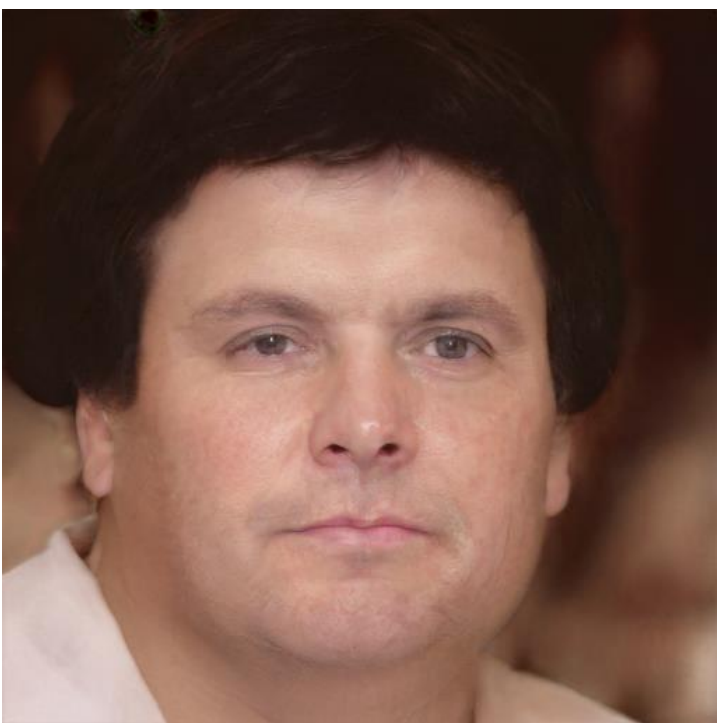

PULSE

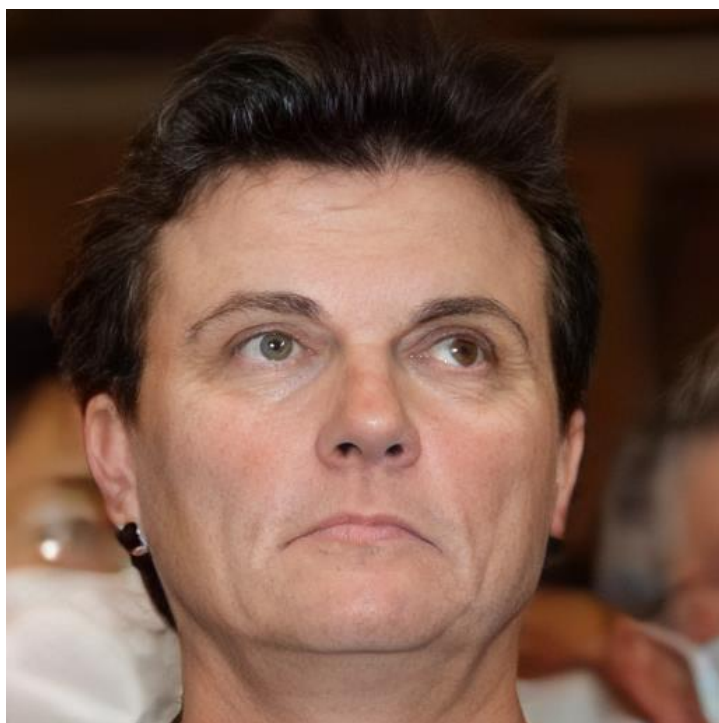

GFP-GAN

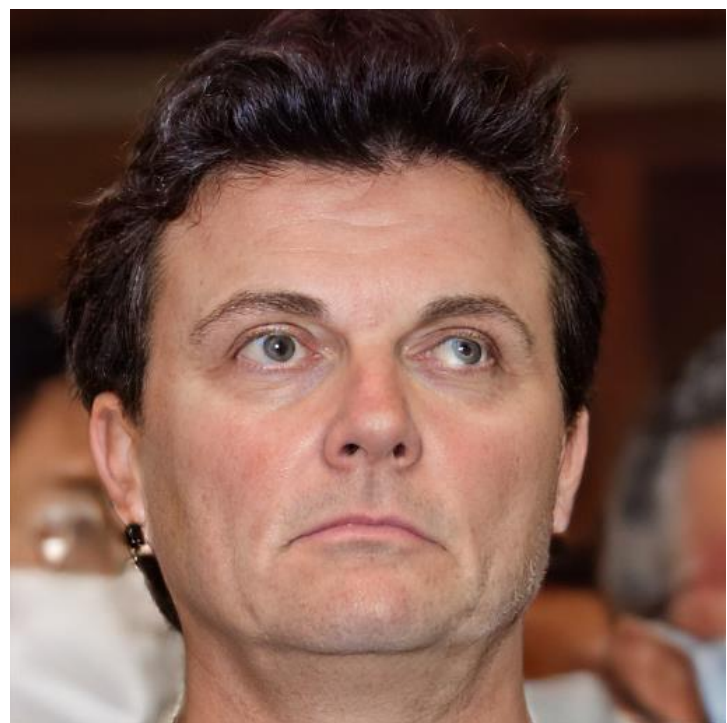

VQFR(ours)

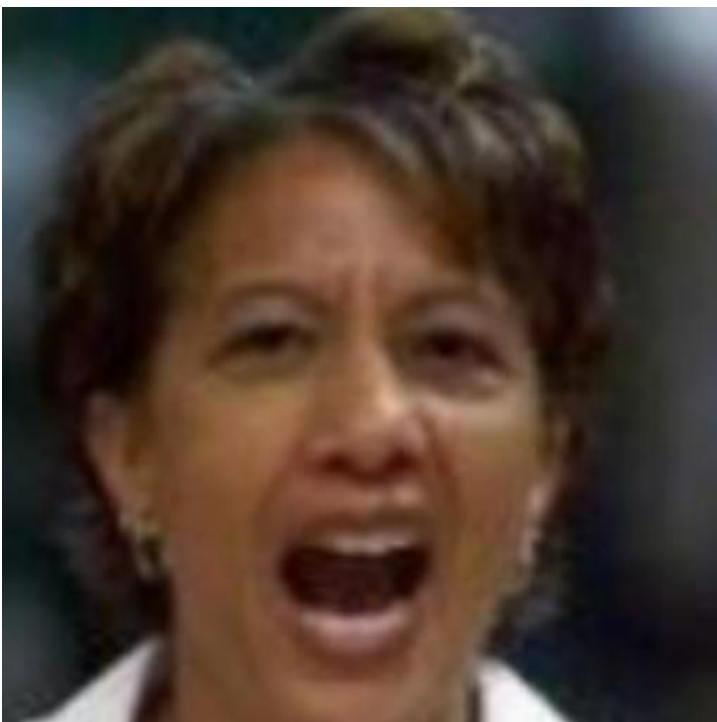

Input

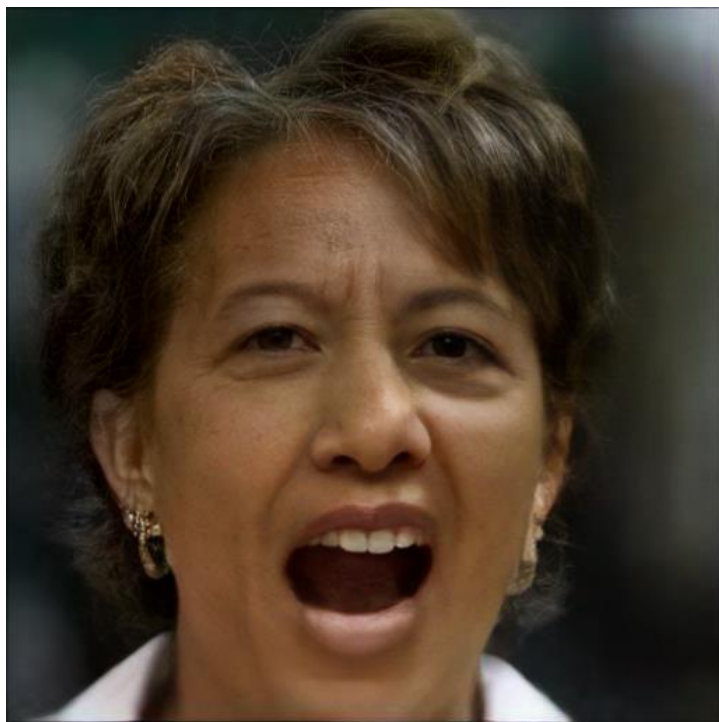

DFDNet

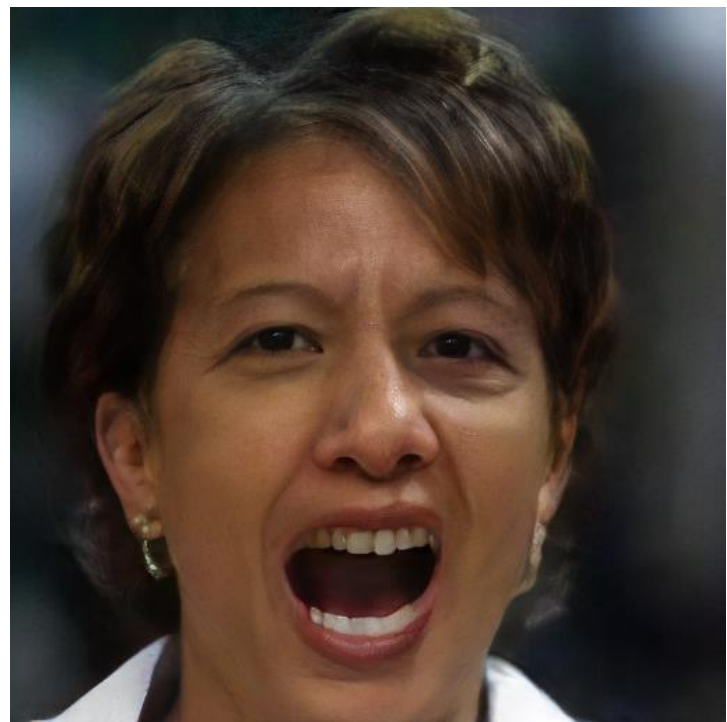

PSFRGAN

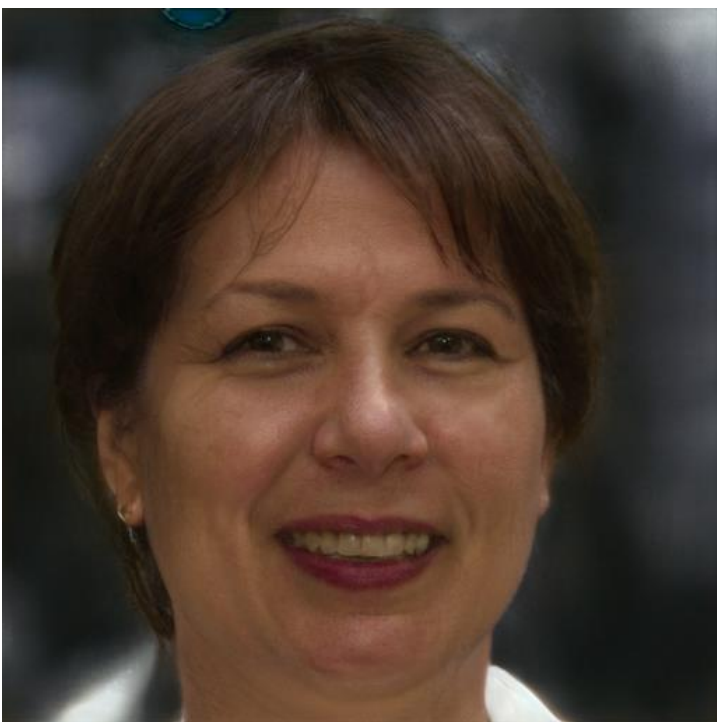

PULSE

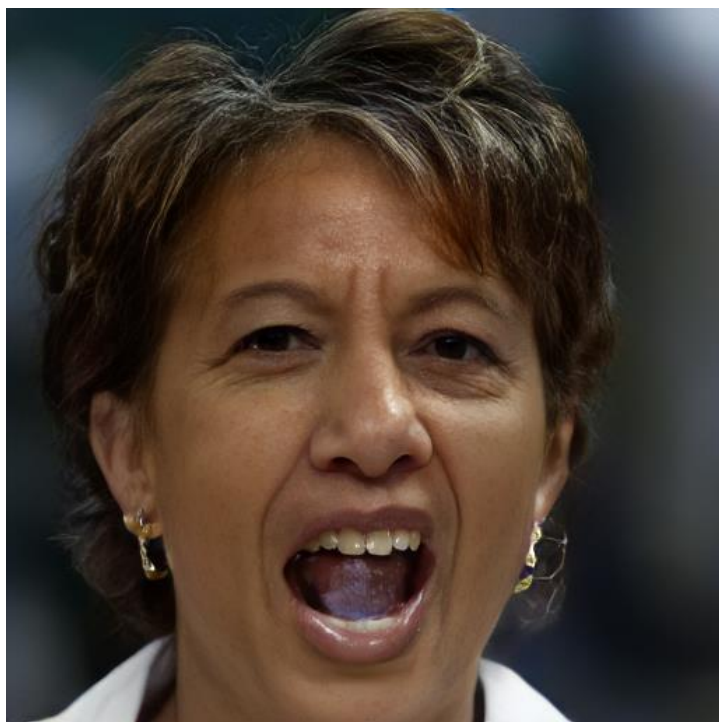

GFP-GAN

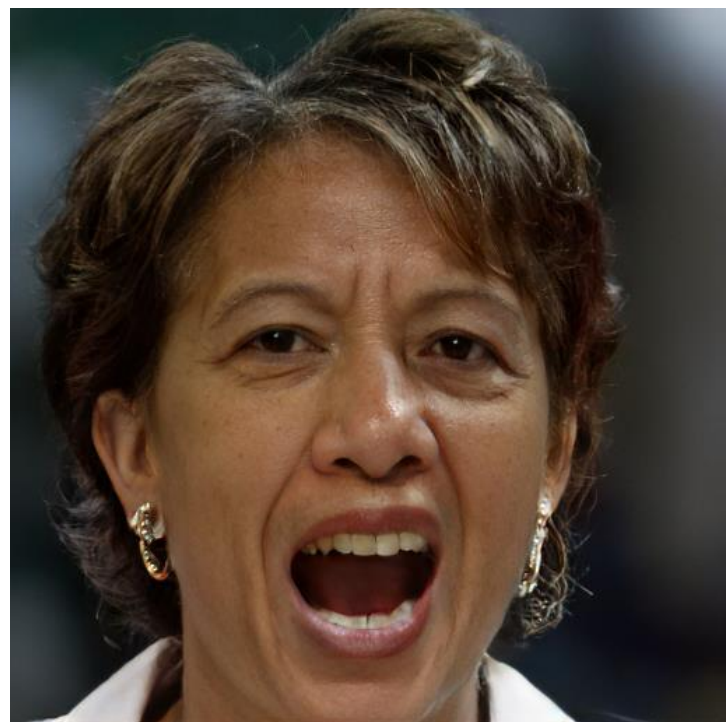

VQFR(ours)
